# Supplementary material for: Comparative analysis of optical character recognition methods for S\'ami texts from the National Library of Norway
Source: arXiv:2501.07300 source file (2025-01-13)
Supplement: Supplementary file 2 [file character_errors.tex]

\begin{tabular}{@{}c@{}c@{}ccc@{}c@{}ccc@{}c@{}ccc@{}c@{}cc@{}}
\toprule
\multicolumn{4}{c}{\textbf{Transkribus}} & \multicolumn{4}{c}{\textbf{Tesseract}} & \multicolumn{4}{c}{\textbf{TrOCR}} & \multicolumn{4}{c}{\textbf{Baseline}} \\
\cmidrule(r){1-4}\cmidrule(lr){5-8}\cmidrule(lr){9-12}\cmidrule(lr){13-16}
\multicolumn{3}{c}{Error} & \# & \multicolumn{3}{c}{Error} & \# & \multicolumn{3}{c}{Error} & \# & \multicolumn{3}{c}{Error} & \# \\
\cmidrule(r){1-3}\cmidrule(lr){4-4}\cmidrule(lr){5-7}\cmidrule(lr){8-8}\cmidrule(lr){9-11}\cmidrule(lr){12-12}\cmidrule(lr){13-15}\cmidrule(l){16-16}
`â' & \(\rightarrow\) & `a' & 8 & `ï' & \(\rightarrow\) & `i' & 18 & `Á' & \(\rightarrow\) & `A' & 5 & `á' & \(\rightarrow\) & `å' & 313 \\
`/' & \(\rightarrow\) & ` ' & 8 & `â' & \(\rightarrow\) & `á' & 17 & `i' & \(\rightarrow\) & `ï' & 5 & `ï' & \(\rightarrow\) & `i' & 137 \\
`i' & \(\rightarrow\) & `ï' & 7 & `' & \(\rightarrow\) & ` ' & 14 & `/' & \(\rightarrow\) & `l' & 4 & `â' & \(\rightarrow\) & `å' & 103 \\
`Á' & \(\rightarrow\) & `A' & 6 & `' & \(\rightarrow\) & `i' & 11 & `Å' & \(\rightarrow\) & `A' & 3 & `–' & \(\rightarrow\) & `-' & 75 \\
`ï' & \(\rightarrow\) & `i' & 5 & `đ' & \(\rightarrow\) & `d' & 11 & `' & \(\rightarrow\) & `j' & 3 & `š' & \(\rightarrow\) & `s' & 72 \\
`š' & \(\rightarrow\) & `' & 4 & `' & \(\rightarrow\) & `á' & 9 & `' & \(\rightarrow\) & ` ' & 3 & `đ' & \(\rightarrow\) & `d' & 48 \\
`Å' & \(\rightarrow\) & `A' & 3 & `Á' & \(\rightarrow\) & `A' & 6 & `j' & \(\rightarrow\) & `i' & 3 & `á' & \(\rightarrow\) & `a' & 46 \\
`Š' & \(\rightarrow\) & `S' & 3 & `â' & \(\rightarrow\) & `å' & 6 & `l' & \(\rightarrow\) & `I' & 3 & `â' & \(\rightarrow\) & `á' & 30 \\
`' & \(\rightarrow\) & `-' & 3 & `l' & \(\rightarrow\) & `I' & 5 & `s' & \(\rightarrow\) & `t' & 3 & `â' & \(\rightarrow\) & `ä' & 26 \\
`đ' & \(\rightarrow\) & `d' & 3 & `s' & \(\rightarrow\) & `S' & 5 & `Å' & \(\rightarrow\) & `Á' & 3 & `č' & \(\rightarrow\) & `c' & 26 \\
\bottomrule
\end{tabular}
